# Supplementary material for: Tools to Explain Neural Networks for Power System Dynamics
Source: arXiv:2608.08048 source file (2026-08-08)
Supplement: Supplementary file 2 [file traj_list.tex]

\def\trajlist{482,413,326,473,295}
